# Supplementary material for: Intensity interferometry for holography with quantum and classical light
Source: arXiv:2301.10068 source file (2023-05-25)
Supplement: Supplementary file 1 [file appendix.tex]

\section*{Supplementary Material}
We make no assumptions about the photon statistics of these input fields for now.
The outputs of the beam splitter are measured using spatially-resolved detectors such as a camera.
Correlations in the intensities at the output of the beam splitter are given by:
\begin{equation}
\braket{\hat{I}_c(x_1)\hat{I}_d(x_2)} = \braket{\hat{E}_c^+(x_1) \hat{E}_c^-(x_1) \hat{E}_d^+(x_2) \hat{E}_d^-(x_2)}
\end{equation}
where $\hat{E}_i^+(x)$ denotes the creation operator in mode $i$ at position $x$.
Note that $[\hat{E}_i^+(x),\hat{E}_i^-(x')]=\delta(x-x')$. 
We can relate this to the inputs using the input-output relation of the beam splitter: $\hat{E}_c = (\hat{E}_a+\hat{E}_b)/\sqrt{2}$ and $\hat{E}_d = (\hat{E}_a-\hat{E}_b)/\sqrt{2}$.
Moreover, we assume that there is a phase in the $b$ mode $\hat{E}^+_b\rightarrow \hat{E}^+_b e^{i\theta}$.
There are in principle 16 terms, but 10 of them (which contain an odd number of creation or anhiliation operators in either input mode) vanish due to the phase average. 
For example, $\int_0^{2\pi} d\theta e^{i\theta} \hat{E}_b^+(x_1) \hat{E}_a^+(x_2) \hat{E}_a^-(x_1) \hat{E}_a^-(x_2) =0$.
We are left with:
\begin{equation}
\begin{split}
\braket{\hat{I}_c(x_1)\hat{I}_d(x_2)} 
&= \frac{1}{4}[\braket{\hat{E}_a^+(x_1) \hat{E}_b^+(x_2) \hat{E}_a^-(x_1) \hat{E}_b^-(x_2)} \\ 
&\quad + \braket{\hat{E}_b^+(x_1) \hat{E}_a^+(x_2) \hat{E}_b^-(x_1) \hat{E}_a^-(x_2)} \\
&\quad + \braket{\hat{E}_a^+(x_1) \hat{E}_a^+(x_2) \hat{E}_a^-(x_1) \hat{E}_a^-(x_2)} \\ 
&\quad + \braket{\hat{E}_b^+(x_1) \hat{E}_b^+(x_2) \hat{E}_b^-(x_1) \hat{E}_b^-(x_2)} \\
&\quad - \braket{\hat{E}_b^+(x_1) \hat{E}_a^+(x_2) \hat{E}_a^-(x_1) \hat{E}_b^-(x_2)} \\
&\quad - \braket{\hat{E}_a^+(x_1) \hat{E}_b^+(x_2) \hat{E}_b^-(x_1) \hat{E}_a^-(x_2)}] \\
&= \frac{1}{4}[\braket{\hat{I}_a(x_1)}\braket{\hat{I}_b(x_2)} + \braket{\hat{I}_a(x_2)}\braket{\hat{I}_b(x_1)} \\ 
&\quad + \braket{\hat{E}_a^+(x_1) \hat{E}_a^+(x_2) \hat{E}_a^-(x_1) \hat{E}_a^-(x_2)} \\ 
&\quad + \braket{\hat{E}_b^+(x_1) \hat{E}_b^+(x_2) \hat{E}_b^-(x_1) \hat{E}_b^-(x_2)} \\
&\quad - \braket{\hat{E}_b^+(x_1) \hat{E}_b^-(x_2)}\braket{\hat{E}_a^+(x_2) \hat{E}_a^-(x_1) } \\
&\quad - \braket{\hat{E}_b^+(x_2) \hat{E}_b^-(x_1)}\braket{\hat{E}_a^+(x_1) \hat{E}_a^-(x_2)}] \\
\end{split}
\end{equation}
The last two terms correspond to the intereference between the possibilities of the photodetection at $x_1$ coming from input $a$ and $b$.
The middle two terms depend on the intensity fluctuations of the signal and reference beams.
Lets assume that the average intensity in both inputs is equal, i.e. $\braket{\hat{I}_a(x)}=\braket{\hat{I}_b(x)}$.
We can re-write the last line of Eq.? in terms of quantities normalized by their energy:
\begin{equation}
\begin{split}
\frac{\braket{\hat{I}_c(x_1)\hat{I}_d(x_2)}}{\braket{\hat{I}(x_1)}\braket{\hat{I}(x_2)}} = \frac{1}{4}\left( 2 + g_a^{(2)}(x_1,x_2) + g_b^{(2)}(x_1,x_2) - 2\mathrm{Re}[g_a^{(1)}(x_2,x_1)g_b^{(1)}(x_1,x_2)]) \right)
\end{split}
\label{eqn:normalized_intensity_correlations}
\end{equation}
We see that the relevance of intensity fluctuations which are given by the second-order correlation functions of the input fields, 
\begin{equation}
g_a^{(2)}(x_1,x_2) = \frac{\braket{\hat{E}_a^+(x_1) \hat{E}_a^+(x_2) \hat{E}_a^-(x_1) \hat{E}_a^-(x_2)}}{\braket{\hat{I}_a(x_1)}\braket{\hat{I}_a(x_2)}}
\end{equation}
The last term in Eq.~\eqref{eqn:normalized_intensity_correlations} is an interference term which depends on the first-order correlation function:
\begin{equation}
g_a^{(1)}(x_2,x_1) = \frac{\braket{\hat{E}_a^+(x_2) \hat{E}_a^-(x_1)}}{[\braket{\hat{I}_a(x_1)}\braket{\hat{I}_a(x_2)}]^{1/2}}
\end{equation}
Note that $g_a^{(1)}(x_2,x_1) = g_a^{(1)}(x_1,x_2)^*$.
The intensity interferometry measurement also probes the spatial coherence function of the input fields which is. 

We can use this expression to obtain the interference visibility dependence on the photon statistics of the input fields.
The reference field will be a coherent state, so $g^{(2)}_{b}(x_1,x_2)=1$.
We will assume that our input fields are in a single pure spatial mode and so $|g^{(1)}_{a,b}(x_1,x_2)|=1$ which can apply to fields with any photon statistics, e.g. single photon or thermal states.
Applying a shear to one of the fields will reveal a cosine modulation between $-1$ and $1$.
Thus the visibility is given by
\begin{equation}
\mathcal{V} = \frac{2}{3+g^{(2)}_{a}(x_1,x_2)}
\end{equation}

% Consider a particular case where the inputs in $a$ and $b$ are spatially uniform besides a shear, i.e. $\hat{E}^-_a(x_1)\rightarrow\hat{E}^-_a$ and $\hat{E}^-_b(x_1)\rightarrow\hat{E}^-_be^{ik_0x_1}$.
% Then, 
% \begin{equation}
% \begin{split}
%     \braket{\hat{I}_c(x_1)\hat{I}_d(x_2)} &= \braket{\hat{I}^2_a} + \braket{\hat{I}^2_b} \\
%     &\quad + 2\braket{\hat{I}_a}\braket{\hat{I}_b}(1-\cos{[k_0(x_2-x_1)]}) 
% \end{split}
% \end{equation}
% For equal input intensities and fluctuations, i.e. $\braket{I_a}=\braket{I_b}$ and $\braket{I^2_a}=\braket{I^2_b}$, the fringe visibility is given by
% \begin{equation}
% \mathcal{V} = \frac{\braket{I}^2}{\braket{I}^2 + \braket{I^2}}.
% \end{equation}
% For thermal states, $\braket{I^2}=2\braket{I}^2 + \braket{I}^{-1}$ and so $\mathcal{V}\rightarrow1/3$ as $\braket{I}\rightarrow \infty$.
% For coherent states, $\braket{I^2}=\braket{I}^2$ and so $\mathcal{V}=1/2$.
% Only non-classical fields permit sub-Poissonian statistics like $\braket{I^2} < \braket{I}^2$, with the limiting case being a photon-number state with $\braket{I^2}=0$ in which case $\mathcal{V}=1$.
